# Supplementary material for: A Mountaineering Strategy to Excited States: Accurate Vertical Transition Energies and Benchmarks for Substituted Benzenes
Source: arXiv:2401.13809 ancillary file (2024-01-24)
Supplement: Supplementary file 1 [file PhenCC3-SI.pdf]

# Supporting Information for
# A Mountaineering Strategy to Excited States: Accurate Vertical Transition Energies and Benchmarks for Substituted Benzenes

Pierre-François Loos† and Denis Jacquemin*,‡,¶

†*Laboratoire de Chimie et Physique Quantiques, Université de Toulouse, CNRS, UPS, France*

‡*Nantes Université, CNRS, CEISAM UMR 6230, F-44000 Nantes, France*

¶*Institut Universitaire de France (IUF), F-75005 Paris, France*

E-mail: Denis.Jacquemin@univ-nantes.fr

# S1 Cartesian coordinates (bohrs)

## S1.1 Aminobenzonitrile – CC3(FC)/cc-pVTZ

| | | | |
|---|---|---|---|
| C | 0.00000000 | 0.00000000 | -3.36820633 |
| C | 2.27829762 | 0.00000000 | -2.01450309 |
| C | -2.27829762 | 0.00000000 | -2.01450309 |
| C | 0.00000000 | 0.00000000 | 1.93909521 |
| C | 2.27351166 | 0.00000000 | 0.59753796 |
| C | -2.27351166 | 0.00000000 | 0.59753796 |
| C | 0.00000000 | 0.00000000 | 4.63257112 |
| N | 0.00000000 | 0.00000000 | -5.94870080 |
| N | 0.00000000 | 0.00000000 | 6.83060124 |
| H | 4.04775542 | 0.00000000 | -3.02611570 |
| H | -4.04775542 | 0.00000000 | -3.02611570 |
| H | 4.03704439 | 0.00000000 | 1.61551747 |
| H | -4.03704439 | 0.00000000 | 1.61551747 |
| H | -1.62177115 | 0.00000000 | -6.91608217 |
| H | 1.62177115 | 0.00000000 | -6.91608217 |

### S1.2 Aniline – CC3(FC)/cc-pVTZ

| | | | |
|---|---|---|---|
| C | 0.00000000 | 0.00000000 | -1.78643569 |
| C | 2.27316118 | 0.00000000 | -0.43457234 |
| C | -2.27316118 | 0.00000000 | -0.43457234 |
| C | 0.00000000 | 0.00000000 | 3.53007775 |
| C | 2.26327651 | 0.00000000 | 2.18912925 |
| C | -2.26327651 | 0.00000000 | 2.18912925 |
| N | 0.00000000 | 0.00000000 | -4.38230793 |
| H | 4.03982526 | 0.00000000 | 3.18807501 |
| H | -4.03982526 | 0.00000000 | 3.18807501 |
| H | 0.00000000 | 0.00000000 | 5.56493193 |
| H | 4.04200589 | 0.00000000 | -1.45016965 |
| H | -4.04200589 | 0.00000000 | -1.45016965 |
| H | -1.62137595 | 0.00000000 | -5.34754284 |
| H | 1.62137595 | 0.00000000 | -5.34754284 |

## S1.3 Benzonitrile – CC3(FC)/cc-pVTZ

| | | | |
|---|---|---|---|
| C | 0.00000000 | 0.00000000 | -3.73018216 |
| C | 0.00000000 | 0.00000000 | -1.02720486 |
| C | 2.28760421 | 0.00000000 | 0.28592358 |
| C | -2.28760421 | 0.00000000 | 0.28592358 |
| C | 0.00000000 | 0.00000000 | 4.22270922 |
| C | 2.28059554 | 0.00000000 | 2.90986462 |
| C | -2.28059554 | 0.00000000 | 2.90986462 |
| N | 0.00000000 | 0.00000000 | -5.92640038 |
| H | 4.03930466 | 0.00000000 | -0.75078588 |
| H | -4.03930466 | 0.00000000 | -0.75078588 |
| H | 4.04556576 | 0.00000000 | 3.92452034 |
| H | -4.04556576 | 0.00000000 | 3.92452034 |
| H | 0.00000000 | 0.00000000 | 6.25892556 |

## S1.4 Chlorobenzene – CC3(FC)/cc-pVTZ

| | | | |
|---|---|---|---|
| Cl | 0.00000000 | 0.00000000 | -4.09694569 |
| C | 0.00000000 | 0.00000000 | -0.80648356 |
| C | 2.28704058 | 0.00000000 | 0.47978453 |
| C | -2.28704058 | 0.00000000 | 0.47978453 |
| C | 0.00000000 | 0.00000000 | 4.42840669 |
| C | 2.27492426 | 0.00000000 | 3.10862132 |
| C | -2.27492426 | 0.00000000 | 3.10862132 |
| H | 4.03299260 | 0.00000000 | -0.56250521 |
| H | -4.03299260 | 0.00000000 | -0.56250521 |
| H | 4.04398612 | 0.00000000 | 4.11768561 |
| H | -4.04398612 | 0.00000000 | 4.11768561 |
| H | 0.00000000 | 0.00000000 | 6.46409111 |

## S1.5 Dimethylaminobenzonitrile – CCSD(T)(FC)/cc-pVTZ

| | | | |
|---|---|---|---|
| C | 0.00000000 | 0.00000000 | -1.96083197 |
| C | 2.27891314 | 0.00000000 | -0.58294740 |
| C | -2.27891314 | 0.00000000 | -0.58294740 |
| C | 0.00000000 | 0.00000000 | 3.37434994 |
| C | 2.26711046 | 0.00000000 | 2.02803761 |
| C | -2.26711046 | 0.00000000 | 2.02803761 |
| C | 0.00000000 | 0.00000000 | 6.06798788 |
| C | 2.36485177 | 0.00000000 | -5.90186899 |
| C | -2.36485177 | 0.00000000 | -5.90186899 |
| N | 0.00000000 | 0.00000000 | -4.53733249 |
| N | 0.00000000 | 0.00000000 | 8.26382999 |
| H | 4.06469412 | 0.00000000 | -1.55103579 |
| H | -4.06469412 | 0.00000000 | -1.55103579 |
| H | 4.03369195 | 0.00000000 | 3.04099978 |
| H | -4.03369195 | 0.00000000 | 3.04099978 |
| H | 1.96836611 | 0.00000000 | -7.91292844 |
| H | -1.96836611 | 0.00000000 | -7.91292844 |
| H | 3.49551175 | -1.67111709 | -5.47003452 |
| H | 3.49551175 | 1.67111709 | -5.47003452 |
| H | -3.49551175 | 1.67111709 | -5.47003452 |
| H | -3.49551175 | -1.67111709 | -5.47003452 |

## S1.6 Dimethylaniline – CCSD(T)(FC)/cc-pVTZ

| | | | |
|---|---|---|---|
| C | 0.00000000 | 0.00000000 | 4.89686867 |
| C | 2.25704297 | 0.00000000 | 3.55138467 |
| C | -2.25704297 | 0.00000000 | 3.55138467 |
| C | 2.27412639 | 0.00000000 | 0.92841898 |
| C | -2.27412639 | 0.00000000 | 0.92841898 |
| C | 0.00000000 | 0.00000000 | -0.44595239 |
| C | 2.36139267 | 0.00000000 | -4.39675011 |
| C | -2.36139267 | 0.00000000 | -4.39675011 |
| N | 0.00000000 | 0.00000000 | -3.03916783 |
| H | 4.05922248 | 0.00000000 | -0.04344476 |
| H | -4.05922248 | 0.00000000 | -0.04344476 |
| H | 4.03670718 | 0.00000000 | 4.54551891 |
| H | -4.03670718 | 0.00000000 | 4.54551891 |
| H | 0.00000000 | 0.00000000 | 6.93154996 |
| H | 1.97020408 | 0.00000000 | -6.40997108 |
| H | -1.97020408 | 0.00000000 | -6.40997108 |
| H | 3.49800498 | -1.66955347 | -3.96565000 |
| H | 3.49800498 | 1.66955347 | -3.96565000 |
| H | -3.49800498 | 1.66955347 | -3.96565000 |
| H | -3.49800498 | -1.66955347 | -3.96565000 |

## S1.7 Fluorobenzene – CC3(FC)/cc-pVTZ

| | | | |
|---|---|---|---|
| F | 0.00000000 | 0.00000000 | -4.15873063 |
| C | 0.00000000 | 0.00000000 | -1.61842149 |
| C | 2.29188824 | 0.00000000 | -0.35805545 |
| C | -2.29188824 | 0.00000000 | -0.35805545 |
| C | 0.00000000 | 0.00000000 | 3.59063853 |
| C | 2.27621870 | 0.00000000 | 2.27153776 |
| C | -2.27621870 | 0.00000000 | 2.27153776 |
| H | 4.02397454 | 0.00000000 | -1.42355397 |
| H | -4.02397454 | 0.00000000 | -1.42355397 |
| H | 4.04329770 | 0.00000000 | 3.28356917 |
| H | -4.04329770 | 0.00000000 | 3.28356917 |
| H | 0.00000000 | 0.00000000 | 5.62589878 |

## S1.8 Nitroaniline – CC3(FC)/cc-pVTZ

| | | | |
|---|---|---|---|
| C | 0.00000000 | 0.00000000 | -4.05915738 |
| C | 2.28068352 | 0.00000000 | -2.70811066 |
| C | -2.28068352 | 0.00000000 | -2.70811066 |
| C | 0.00000000 | 0.00000000 | 1.19144079 |
| C | 2.28308329 | 0.00000000 | -0.09681843 |
| C | -2.28308329 | 0.00000000 | -0.09681843 |
| N | 0.00000000 | 0.00000000 | 3.94052757 |
| N | 0.00000000 | 0.00000000 | -6.63741535 |
| O | 2.04948184 | 0.00000000 | 5.01410797 |
| O | -2.04948184 | 0.00000000 | 5.01410797 |
| H | 4.04799128 | 0.00000000 | -3.72195018 |
| H | -4.04799128 | 0.00000000 | -3.72195018 |
| H | 4.02032559 | 0.00000000 | 0.95557275 |
| H | -4.02032559 | 0.00000000 | 0.95557275 |
| H | -1.62132329 | 0.00000000 | -7.60488781 |
| H | 1.62132329 | 0.00000000 | -7.60488781 |

## S1.9 Nitrobenzene – CC3(FC)/cc-pVTZ

| | | | |
|---|---|---|---|
| C | 0.00000000 | 0.00000000 | -0.33719774 |
| C | 2.29667056 | 0.00000000 | 0.92138137 |
| C | -2.29667056 | 0.00000000 | 0.92138137 |
| C | 0.00000000 | 0.00000000 | 4.85826496 |
| C | 2.28247086 | 0.00000000 | 3.54756893 |
| C | -2.28247086 | 0.00000000 | 3.54756893 |
| N | 0.00000000 | 0.00000000 | -3.11429157 |
| O | -2.05476165 | 0.00000000 | -4.18095202 |
| O | 2.05476165 | 0.00000000 | -4.18095202 |
| H | 4.02347357 | 0.00000000 | -0.14769848 |
| H | -4.02347357 | 0.00000000 | -0.14769848 |
| H | 4.04624818 | 0.00000000 | 4.56388578 |
| H | -4.04624818 | 0.00000000 | 4.56388578 |
| H | 0.00000000 | 0.00000000 | 6.89454456 |

## S1.10 Nitropyridine N-Oxide – CCSD(T)(FC)/cc-pVTZ

| | | | |
|---|---|---|---|
| C | 0.00000000 | 0.00000000 | -1.21738204 |
| C | 2.26825255 | 0.00000000 | 0.09038008 |
| C | -2.26825255 | 0.00000000 | 0.09038008 |
| C | 2.22988276 | 0.00000000 | 2.68605086 |
| C | -2.22988276 | 0.00000000 | 2.68605086 |
| N | 0.00000000 | 0.00000000 | -3.96704616 |
| N | 0.00000000 | 0.00000000 | 4.00601244 |
| O | 0.00000000 | 0.00000000 | 6.38961931 |
| O | -2.05398155 | 0.00000000 | -5.02438491 |
| O | 2.05398155 | 0.00000000 | -5.02438491 |
| H | 4.03491913 | 0.00000000 | -0.90939267 |
| H | -4.03491913 | 0.00000000 | -0.90939267 |
| H | 3.88274506 | 0.00000000 | 3.86446617 |
| H | -3.88274506 | 0.00000000 | 3.86446617 |

### S1.11 Phenolate – CC3(FC)/cc-pVTZ

| | | | |
|---|---|---|---|
| C | 0.00000000 | 0.00000000 | -1.94817868 |
| C | 2.27737723 | 0.00000000 | -0.45104645 |
| C | -2.27737723 | 0.00000000 | -0.45104645 |
| C | 0.00000000 | 0.00000000 | 3.54287236 |
| C | 2.25856599 | 0.00000000 | 2.16672471 |
| C | -2.25856599 | 0.00000000 | 2.16672471 |
| O | 0.00000000 | 0.00000000 | -4.33677175 |
| H | 4.04811102 | 0.00000000 | -1.47084405 |
| H | -4.04811102 | 0.00000000 | -1.47084405 |
| H | 4.04319440 | 0.00000000 | 3.17158878 |
| H | -4.04319440 | 0.00000000 | 3.17158878 |
| H | 0.00000000 | 0.00000000 | 5.58190673 |

## S1.12 Pyranone – CC3(FC)/cc-pVTZ

| | | | |
|---|---|---|---|
| C | 0.00000000 | 0.00000000 | -2.03875103 |
| C | 2.29857501 | 0.00000000 | -0.50612872 |
| C | -2.29857501 | 0.00000000 | -0.50612872 |
| C | 2.18356567 | 0.00000000 | 2.02781371 |
| C | -2.18356567 | 0.00000000 | 2.02781371 |
| O | 0.00000000 | 0.00000000 | 3.36810442 |
| O | 0.00000000 | 0.00000000 | -4.35224344 |
| H | 3.80117763 | 0.00000000 | 3.26042029 |
| H | -3.80117763 | 0.00000000 | 3.26042029 |
| H | 4.10758504 | 0.00000000 | -1.43183287 |
| H | -4.10758504 | 0.00000000 | -1.43183287 |
